# Supplementary material for: Weighted Ensemble Self-Supervised Learning
Source: arXiv:2211.09981 source file (2023-04-09)
Supplement: Supplementary file 1 [file likelihood_teacher.tex]

\section{Discussion on the conjectured relationship between $\nu$ and $t$}
